# Supplementary material for: FedCTR: Federated Native Ad CTR Prediction with Multi-Platform User Behavior Data
Source: arXiv:2007.12135 source file (2020-07-23)
Supplement: Supplementary file 1 [file supplement.tex]

\section*{Supplementary Materials}

\subsection*{Hyperparameter Settings}

The complete hyperparameter settings are listed in Table~\ref{hyper}.

\begin{table}[h]
\centering
%\resizebox{1.0\linewidth}{!}{
\begin{tabular}{|l|c|}
\hline
\multicolumn{1}{|c|}{\textbf{Hyperparameters}}& \textbf{Value} \\ \hline
word embedding dim.                     & 300            \\ 
\# self-attention heads                  & 16             \\
output dim. of each head               & 16            \\
dropout                                      & 0.2            \\
$\lambda_{LDP}$                                  & 0.01            \\
$\lambda_{DP}$                                  & 0.005            \\
optimizer                                    & Adam           \\
learning rate                                & 1e-3           \\
batch size                                   & 30    \\     \hline
\end{tabular}
%}
\caption{Detailed hyperparameter settings.}\label{hyper}
\end{table}

\subsection*{Detailed Dataset Statistics}
The detailed statistics of the \textit{Ads} and \textit{News} datasets are shown in Table~\ref{dataset2}.

\begin{table}[h]
\centering
\resizebox{0.48\textwidth}{!}{
\begin{tabular}{lrlr}
\hline
\multicolumn{4}{c}{Ads}                                                           \\ \hline
\#users                    & 100,000   & avg. \#words per ad title       & 3.73   \\
\#ads                      & 8,105     & avg. \#words per ad description & 15.31  \\
\#ad click behaviors       & 345,264   & avg. \#words per search query   & 4.64   \\
\#ad non-click behaviors   & 345,264   & avg. \#words per webpage title  & 10.84  \\
avg. \#queries per user    & 50.69     & avg. \#webpages per user        & 210.09 \\ \hline
\multicolumn{4}{c}{News}                                                          \\ \hline
\#users                    & 10,000    & avg. \#queries per user         & 92.30  \\
\#news                     & 42,255    & avg. \#webpages per user        & 81.39  \\
\#impressions              & 360,428   & avg. \#words per news title     & 11.29  \\
\#news click behaviors     & 503,698   & avg. \#words per search query   & 3.25   \\
\#news non-click behaviors & 9,970,795 & avg. \#words per webpage title  & 9.01   \\
 \hline
\end{tabular}
}\caption{Detailed statistics of the \textit{Ads} and \textit{News} datasets.}\label{dataset2}
\end{table}

\subsection*{Ideal Performance of Baseline Methods}
Here we report the ideal performance of baseline methods using
the centralized storage of behavior data from different platforms.
The results under different ratios of training data are summarized
in Tables~\ref{table.performanceideal} and~\ref{table.performance2ideal}.
Since user behavior data is
highly privacy-sensitive and usually cannot be centrally stored or exchanged among different platforms.
Thus, those baseline methods based on centralized data storage cannot achieve the ideal performance due to privacy reasons.
\begin{table}[!t]

\resizebox{0.48\textwidth}{!}{
\begin{tabular}{ccccccc}
\Xhline{1.5pt}
\multirow{2}{*}{\textbf{Methods}} & \multicolumn{2}{c}{25\%}                    & \multicolumn{2}{c}{50\%}                    & \multicolumn{2}{c}{100\%}                   \\ \cline{2-7} 
                                  & AUC                  & AP                   & AUC                  & AP                   & AUC                  & AP                   \\ \hline
LR*               & 60.82  &  57.38  &  61.44 &  58.60 & 62.04 &  59.20\\
LibFM*           & 61.59  &  58.13  &  61.91 &  59.17 & 62.47 &  59.99\\
Wide\&Deep*     & 62.10  &  59.75  &  62.35 &  59.87 & 62.79 &  60.28\\
PNN*              & 62.54  &  60.12  &  62.73 &  60.29 & 62.87 &  60.41\\
DSSM*           & 62.23  &  59.66  &  62.50 &  59.85 & 62.85 &  60.37\\
DeepFM*         & 61.88  &  59.47  &  62.05 &  59.77 & 62.72 &  60.24\\
NativeCTR*         & 62.88  &  60.69  &  63.01 &  60.88 & 63.39 &  61.17\\ \hline
FedCTR               & 63.95  &  61.82  &  64.20 &  62.13 & 64.54 &  62.50 \\
 \Xhline{1.5pt}
\end{tabular}
}
\caption{Results on the \textit{Ads} dataset. * means the ideal performance under centralized user behavior data from different platforms.} \label{table.performanceideal}
\end{table}

\begin{table}[!t]

\resizebox{0.48\textwidth}{!}{
\begin{tabular}{ccccccc}
\Xhline{1.5pt}
\multirow{2}{*}{\textbf{Methods}} & \multicolumn{2}{c}{25\%}                    & \multicolumn{2}{c}{50\%}                    & \multicolumn{2}{c}{100\%}                   \\ \cline{2-7} 
                                  & AUC                  & \small{nDCG@10}                   & AUC                  & \small{nDCG@10}                    & AUC                  & \small{nDCG@10}                    \\ \hline

LibFM*                  &   56.66   &   35.91  &  57.02  &  36.73  &  57.80  &  37.26 \\
EBNR*                   &   61.24   &   39.54  &  61.44  &  39.56  &  61.95  &  40.12 \\
DKN*                    &   60.38   &   38.94  &  60.76  &  39.20  &  61.37  &  39.89 \\
DAN*                    &   60.84   &   39.47  &  61.56  &  39.75  &  62.22  &  40.08 \\
NPA*                    &   61.75   &   39.76  &  62.36  &  40.38  &  62.98  &  40.57 \\ 
NRMS*                   &   62.02   &   39.89  &  62.74  &  40.44  &  63.37  &  41.04 \\ \hline
FedCTR                  &   62.33   &   40.03  &  63.07  &  40.78  &  63.51  &  41.20 \\
 \Xhline{1.5pt}
\end{tabular}
}
 \caption{Results on the \textit{News} dataset. * means the ideal performance under centralized user behavior data from different platforms.} \label{table.performance2ideal}
 
\end{table}

\subsection*{Effect of Aggregator and CTR Predictor}\label{exp.model}
 
\begin{figure}[!t]
  \centering
  \subfigure[\textit{Ads}.]{
    \includegraphics[height=1.1in]{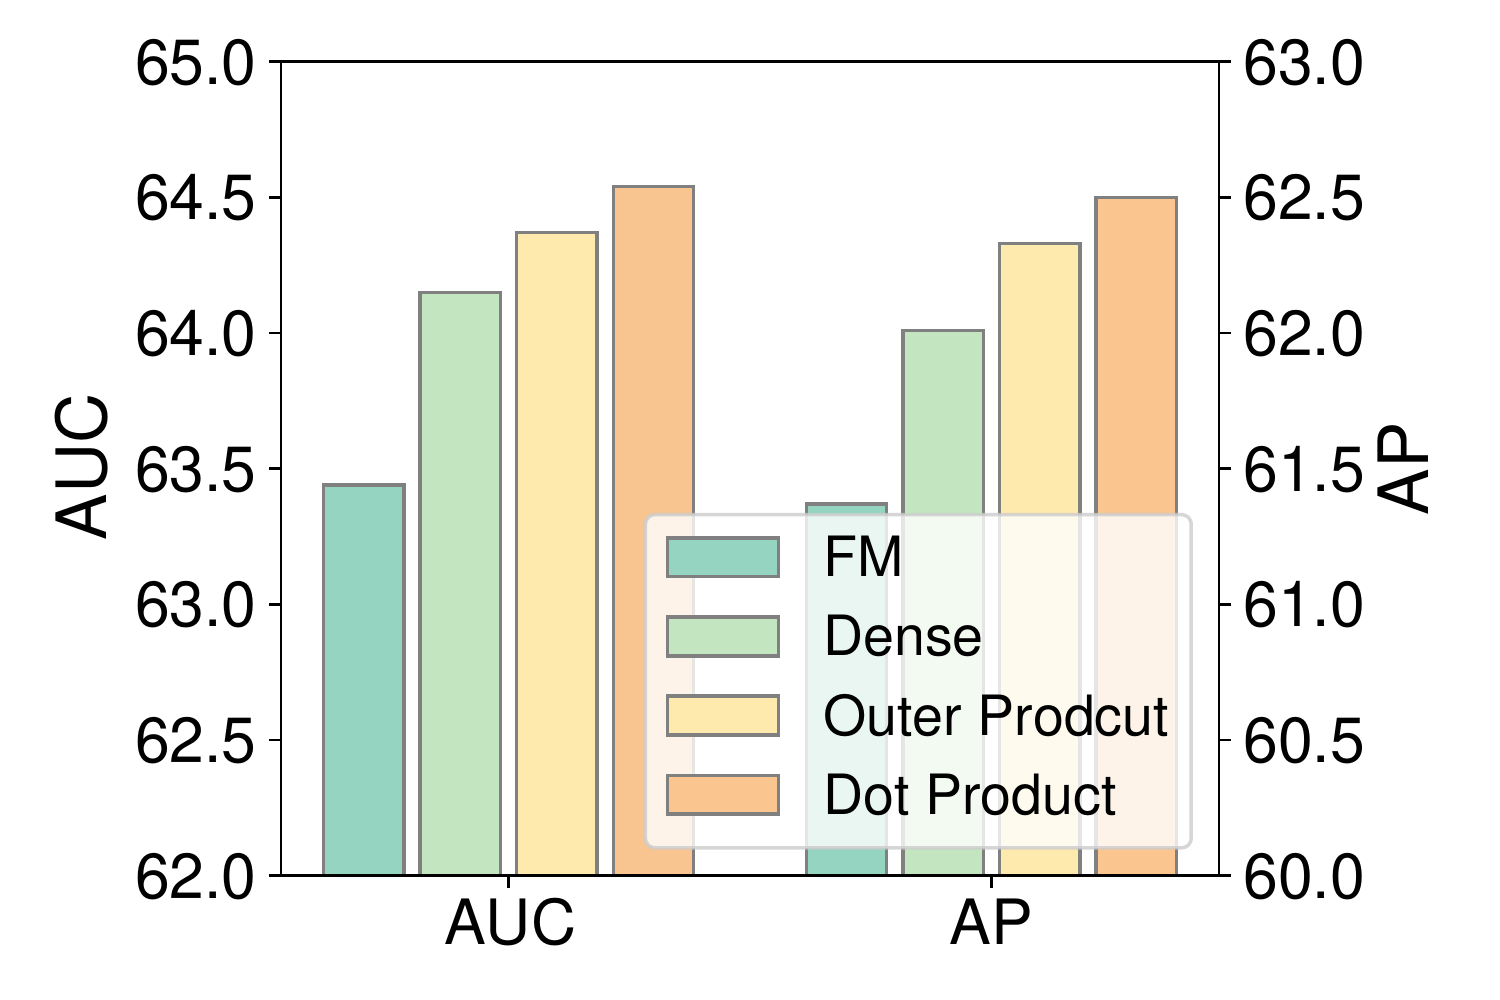}
 
  }
    \subfigure[\textit{News}.]{
      \includegraphics[height=1.1in]{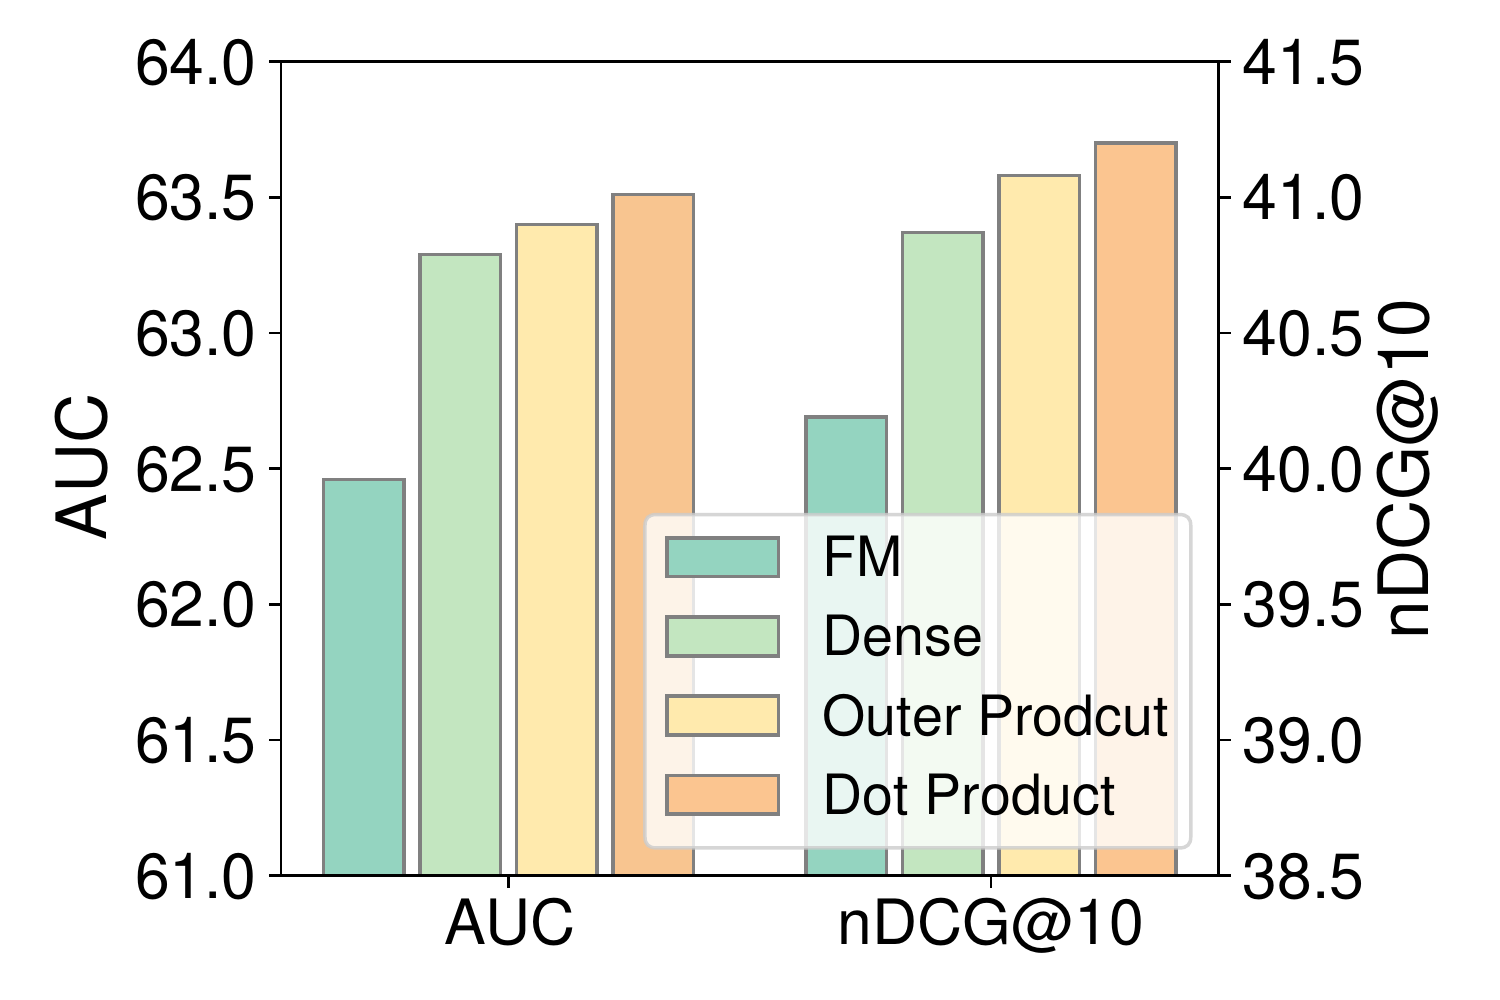}
 
  }
  \caption{Different  CTR predictor models.}  \label{fig.predictor}
\end{figure}

\begin{figure}[!t]
  \centering
  \subfigure[\textit{Ads}.]{
    \includegraphics[height=1.1in]{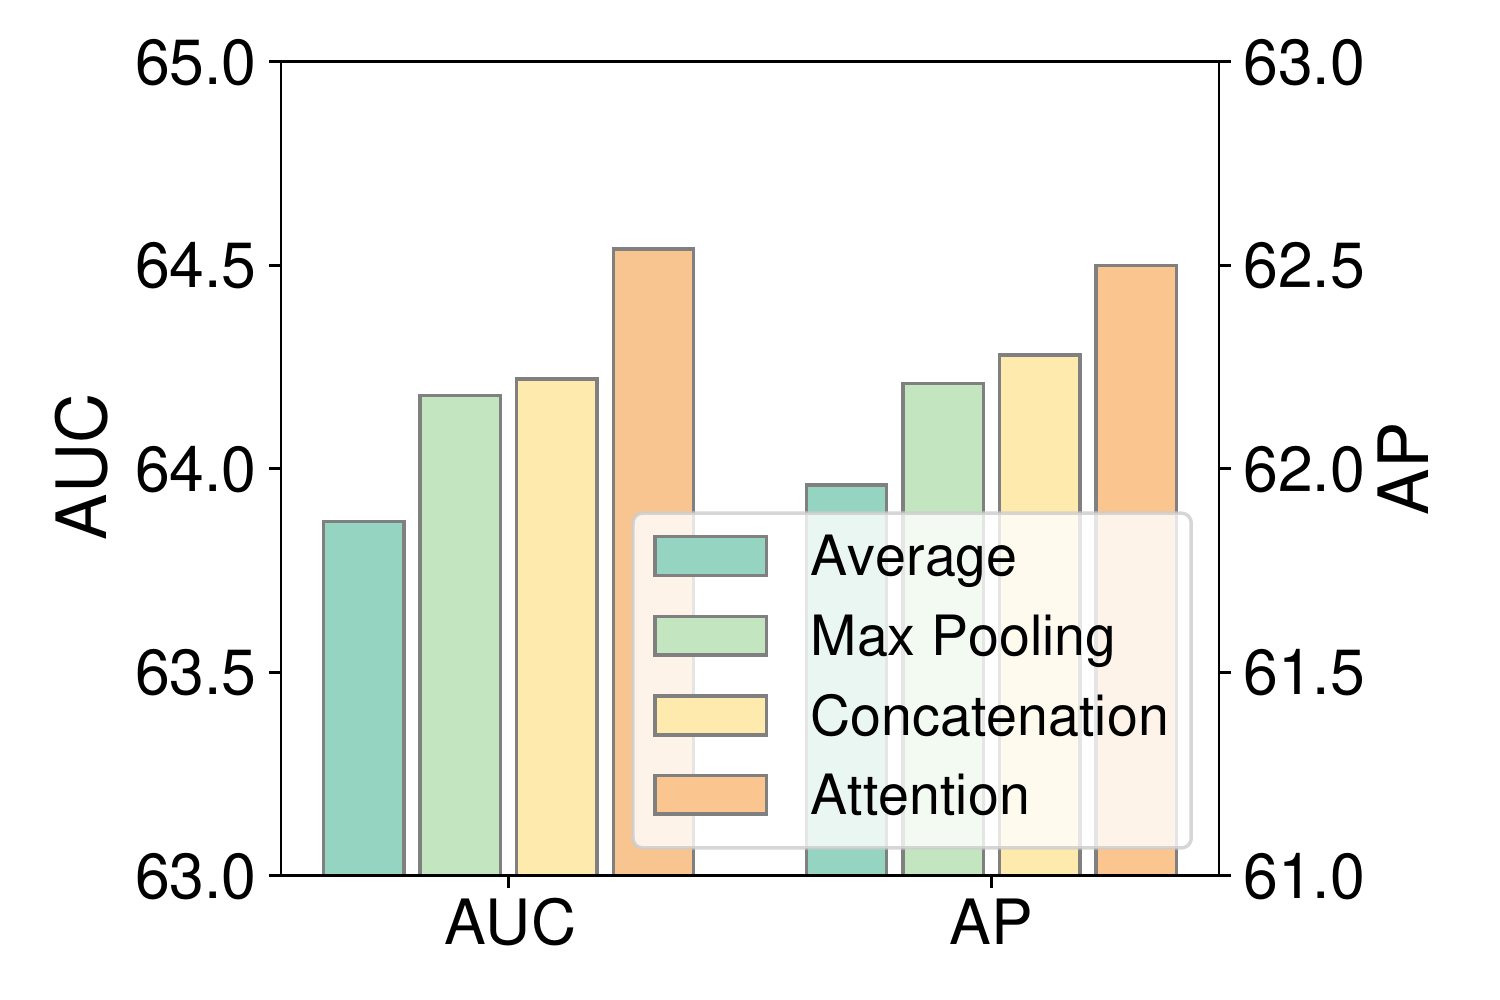}
 
  }
    \subfigure[\textit{News}.]{
      \includegraphics[height=1.1in]{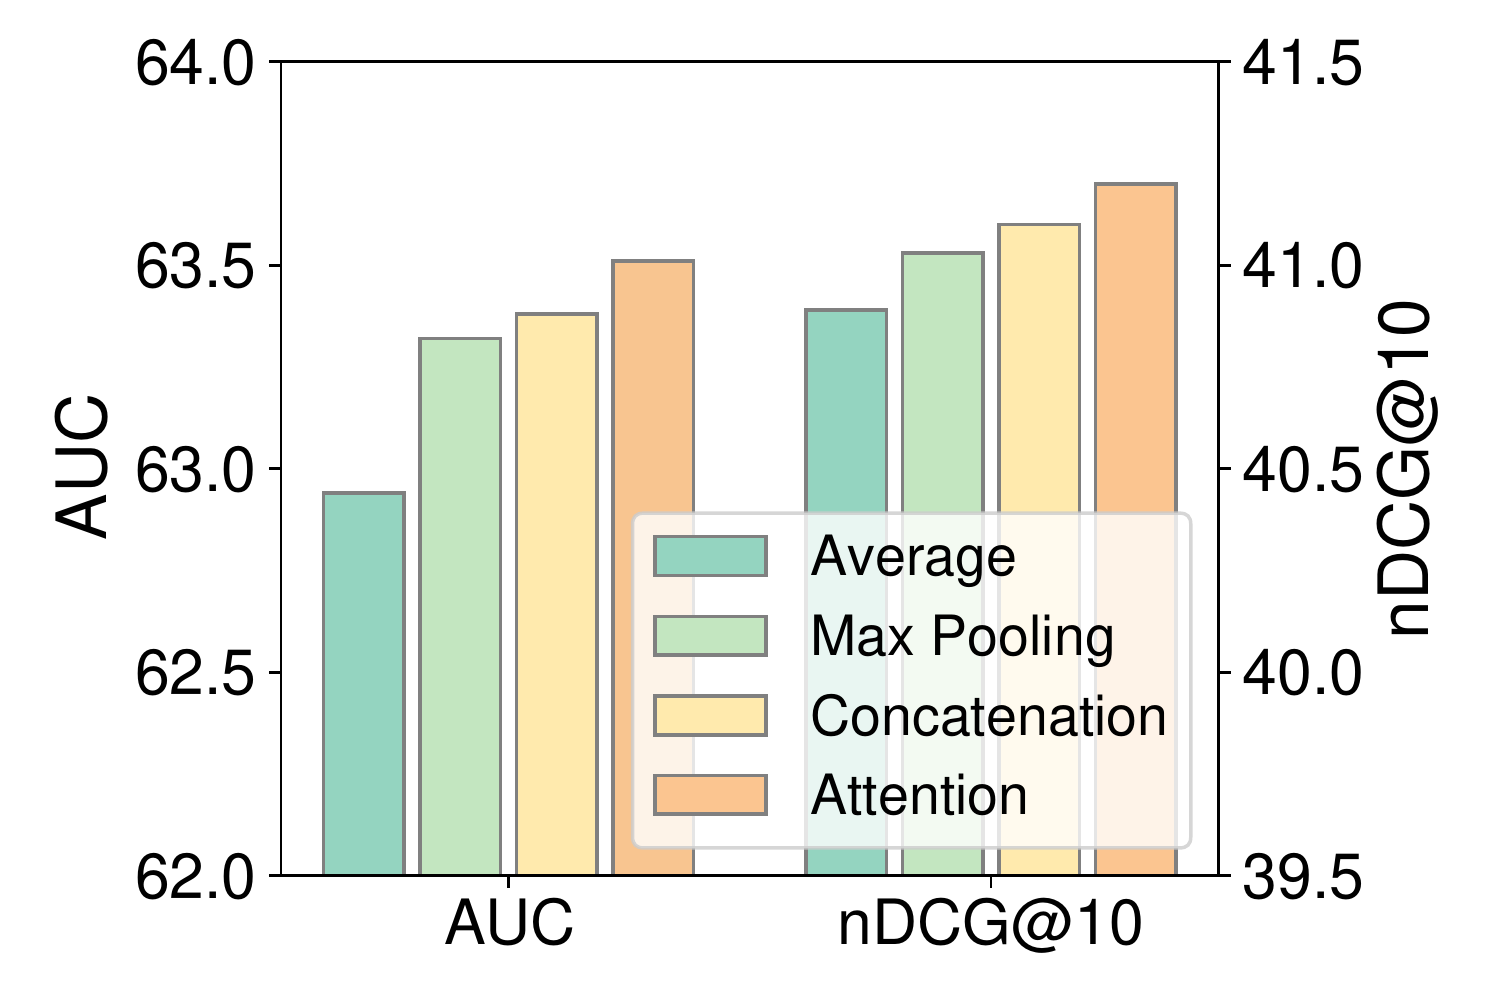}
 
  }
  \caption{Different aggregator models.}  \label{fig.aggregator}
\end{figure}

We verify the effectiveness of the aggregator and CTR predictor models.
First, we compare different CTR prediction models like factorization machine (FM)~\cite{guo2017deepfm}, dense layers, outer product~\cite{he2018outer} and dot product~\cite{an2019neural}, and the results are shown in Fig.~\ref{fig.predictor}.
From Fig.~\ref{fig.predictor}, we find the performance of FM is not optimal.
This may be because FM mainly models the interactions between the elements in two vectors rather than the vector similarity.
In addition, we find that using a dense layer is not optimal.
This may be because in a dense layer the relatedness between the user and ad embeddings is not considered.
Besides, it is interesting that dot product achieves the best performance.
This may be because it is more suitable for modeling the similarity between user and ad embeddings than other compared methods such as outer-product.
Thus, we prefer dot product for its effectiveness and  efficiency.

Then, we compare different models for user embedding aggregation, including attention network, average pooling, max pooling and concatenation.
The results are shown in Fig.~\ref{fig.aggregator}. 
We find that average pooling is sub-optimal for aggregation, since it cannot distinguish the informativeness of different local user embeddings.
In addition, max pooling is also not optimal, since it only keeps the most salient features.
Moreover, although concatenating user embeddings can keep more information, it is inferior to using attention mechanism due to its lack of informativeness modeling.
Thus, we use an attention network to implement the aggregator in the user server.

\subsection*{Complementary Results on the  \textit{News} dataset}

\begin{figure}[!t]
  \centering
  \subfigure[Platform number.]{ 
    \includegraphics[width=0.22\textwidth]{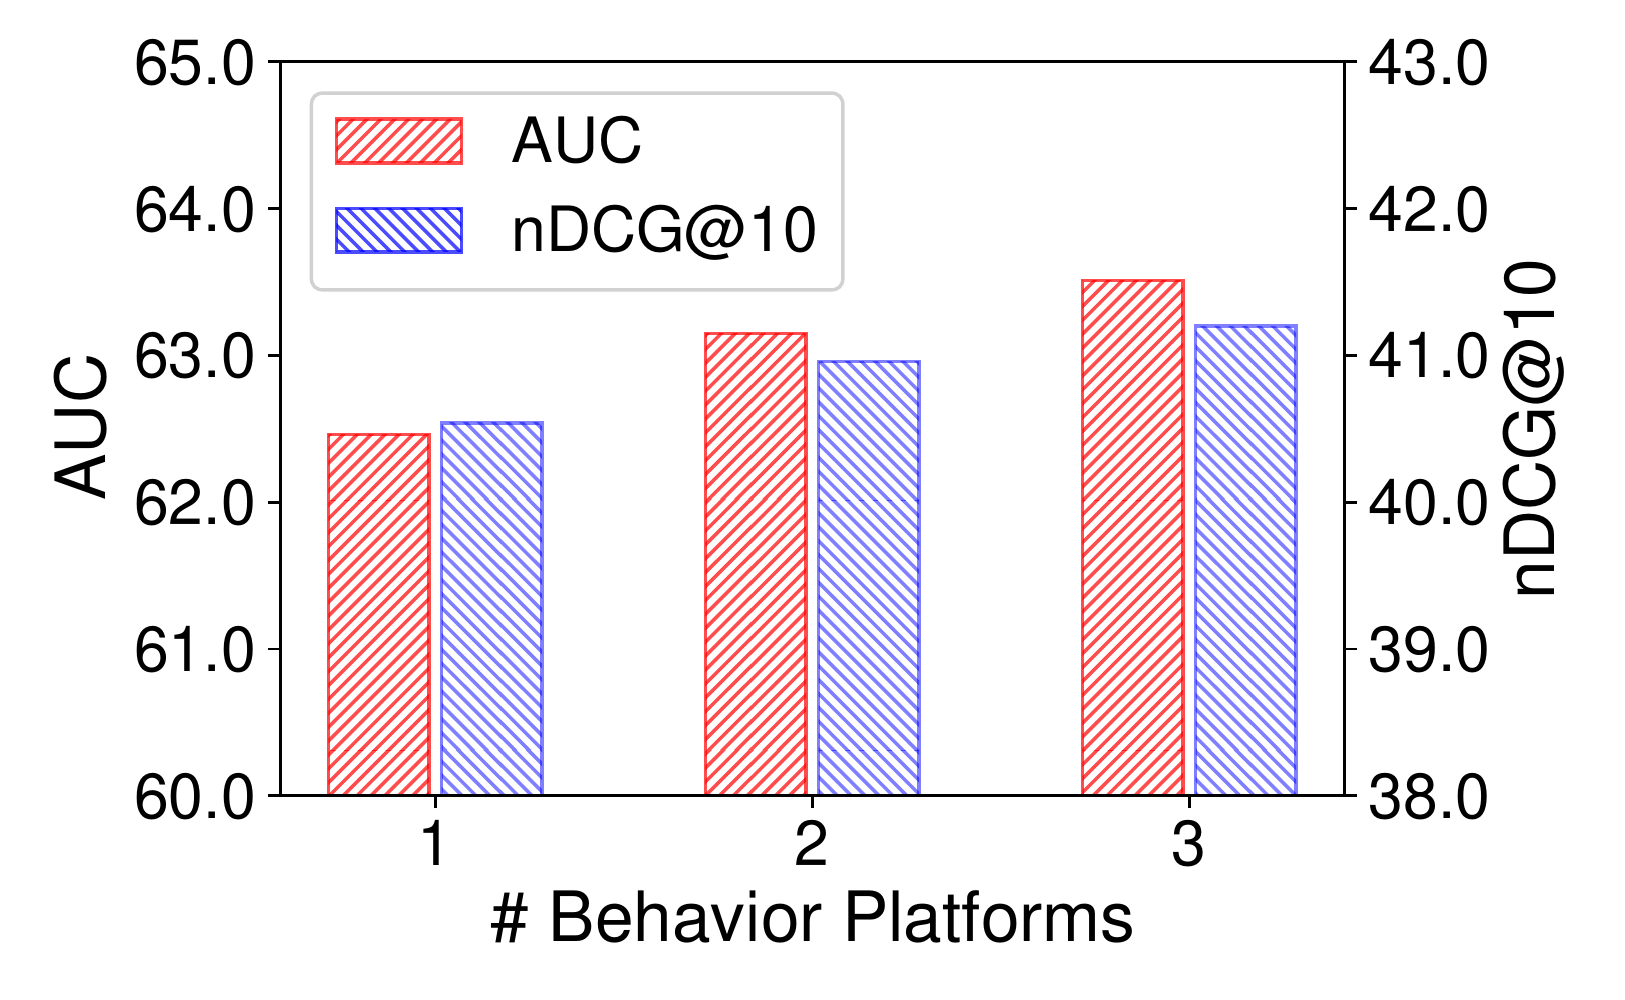}
}
\subfigure[User behavior number.]{    
    \includegraphics[width=0.22\textwidth]{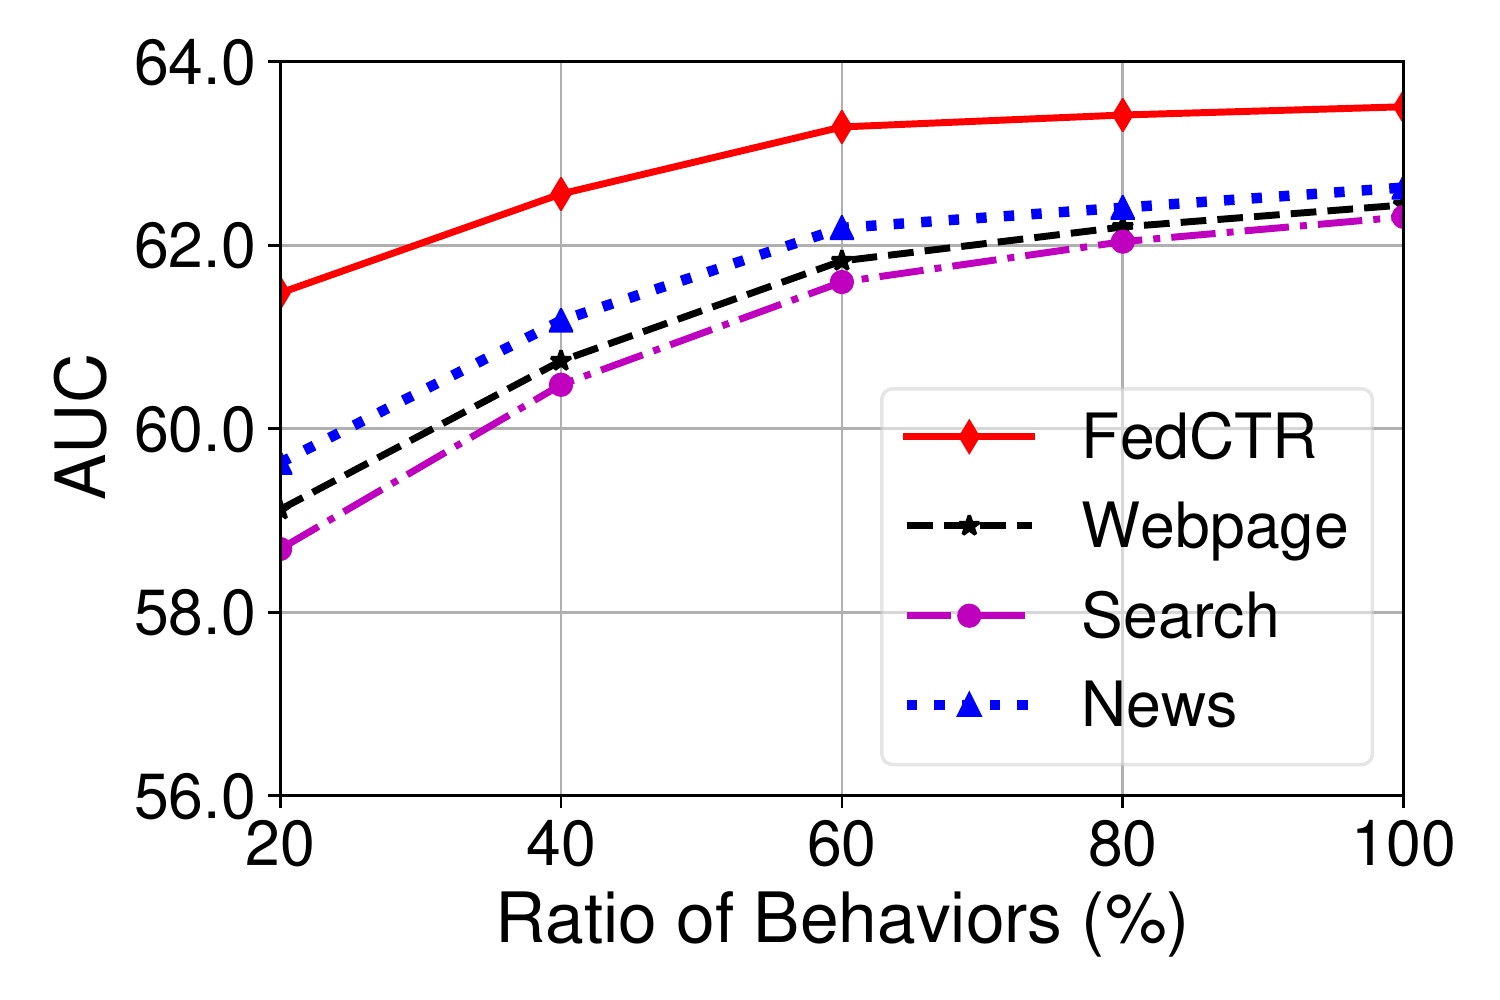}
}

  \caption{Effectiveness of multi-platform behaviors.} \label{fig.behavior2}

\end{figure}

\begin{figure}[!t]
  \centering
  \subfigure[Local embedding.]{
    \includegraphics[width=0.22\textwidth]{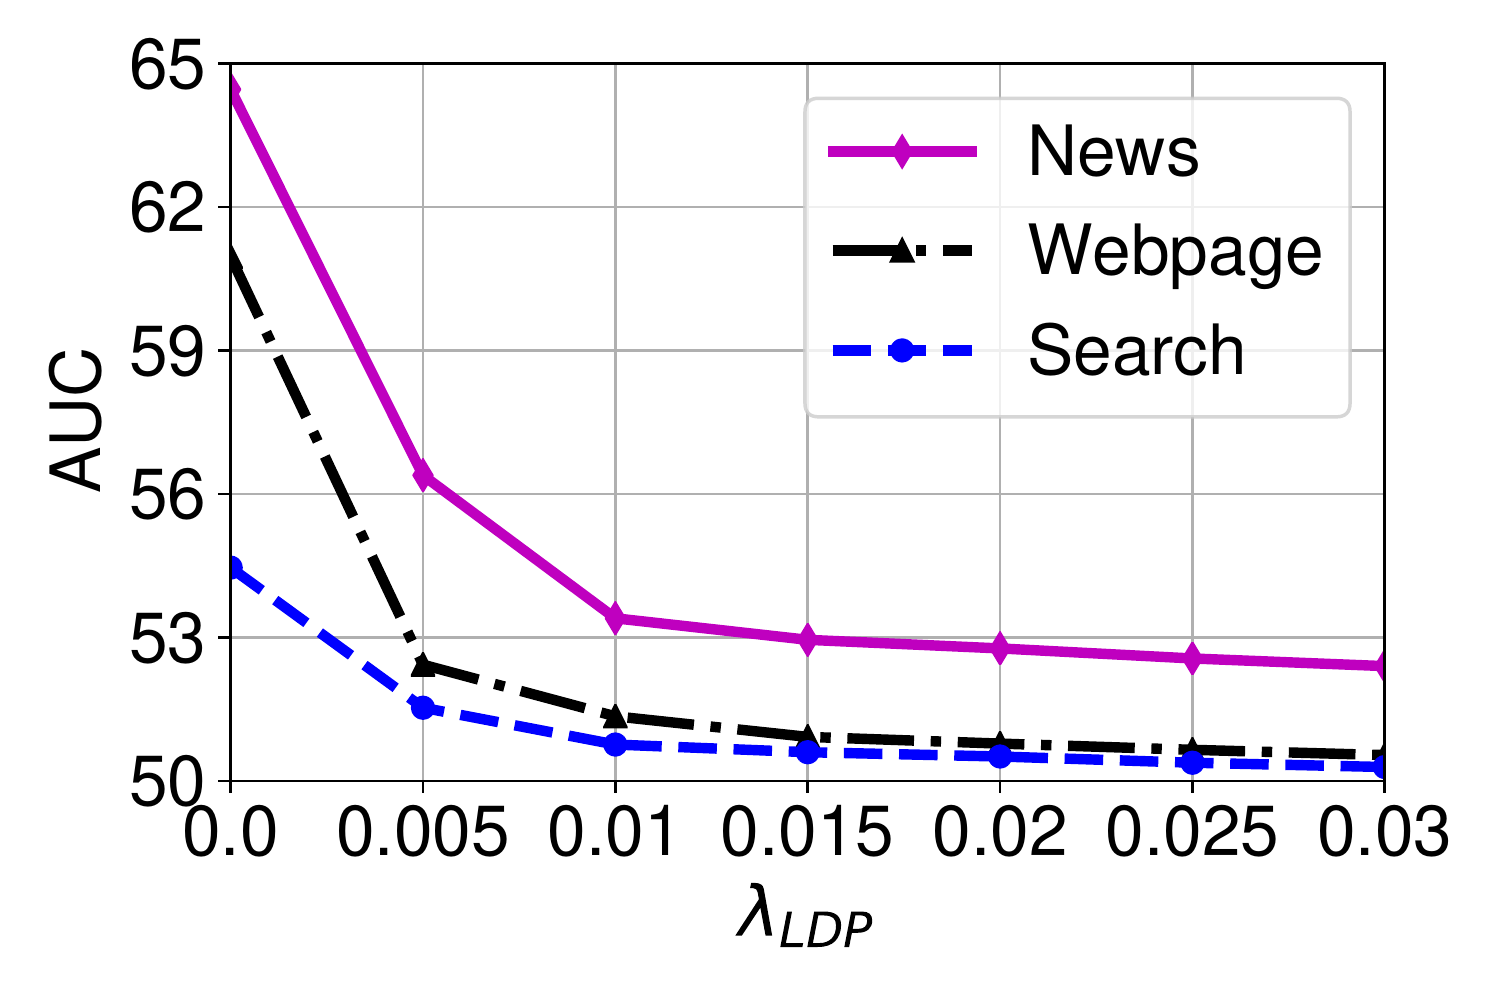}  
    }
    \subfigure[Aggregated embedding.]{
  \includegraphics[width=0.22\textwidth]{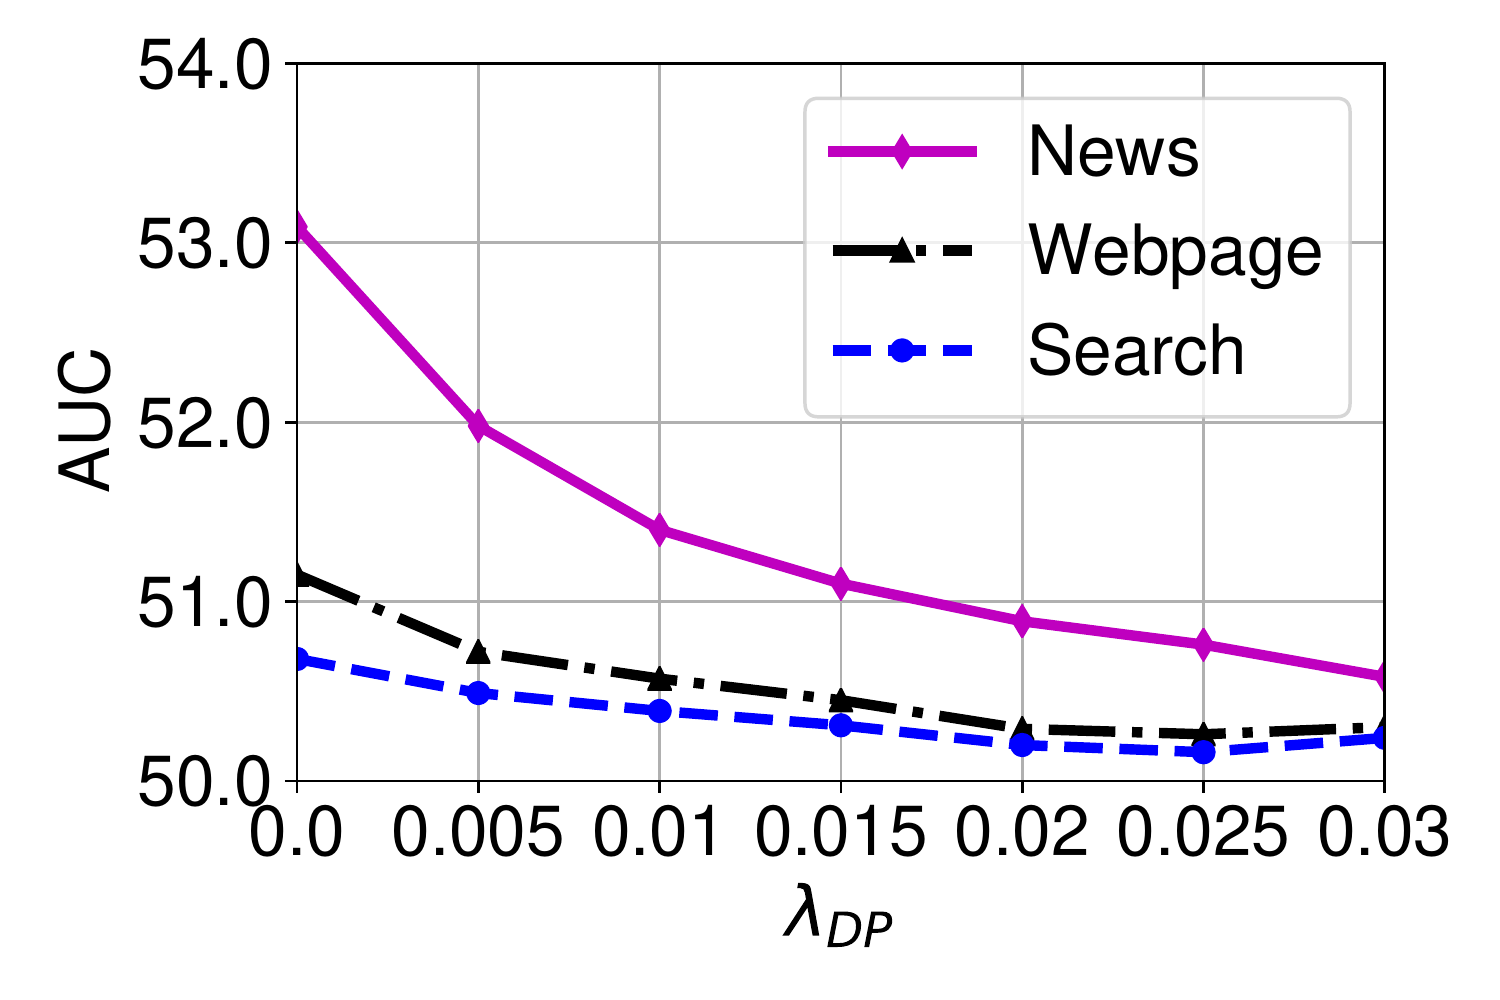}   
    } 
  \caption{Privacy protection of local and aggregated user embedding under different $\lambda_{LDP}$ and $\lambda_{DP}$ values. Lower AUC indicates better privacy protection.} \label{fig.attack3}
\end{figure}
\begin{figure}[!t]
  \centering
  \subfigure[$\lambda_{LDP}$.]{
    \includegraphics[width=0.21\textwidth]{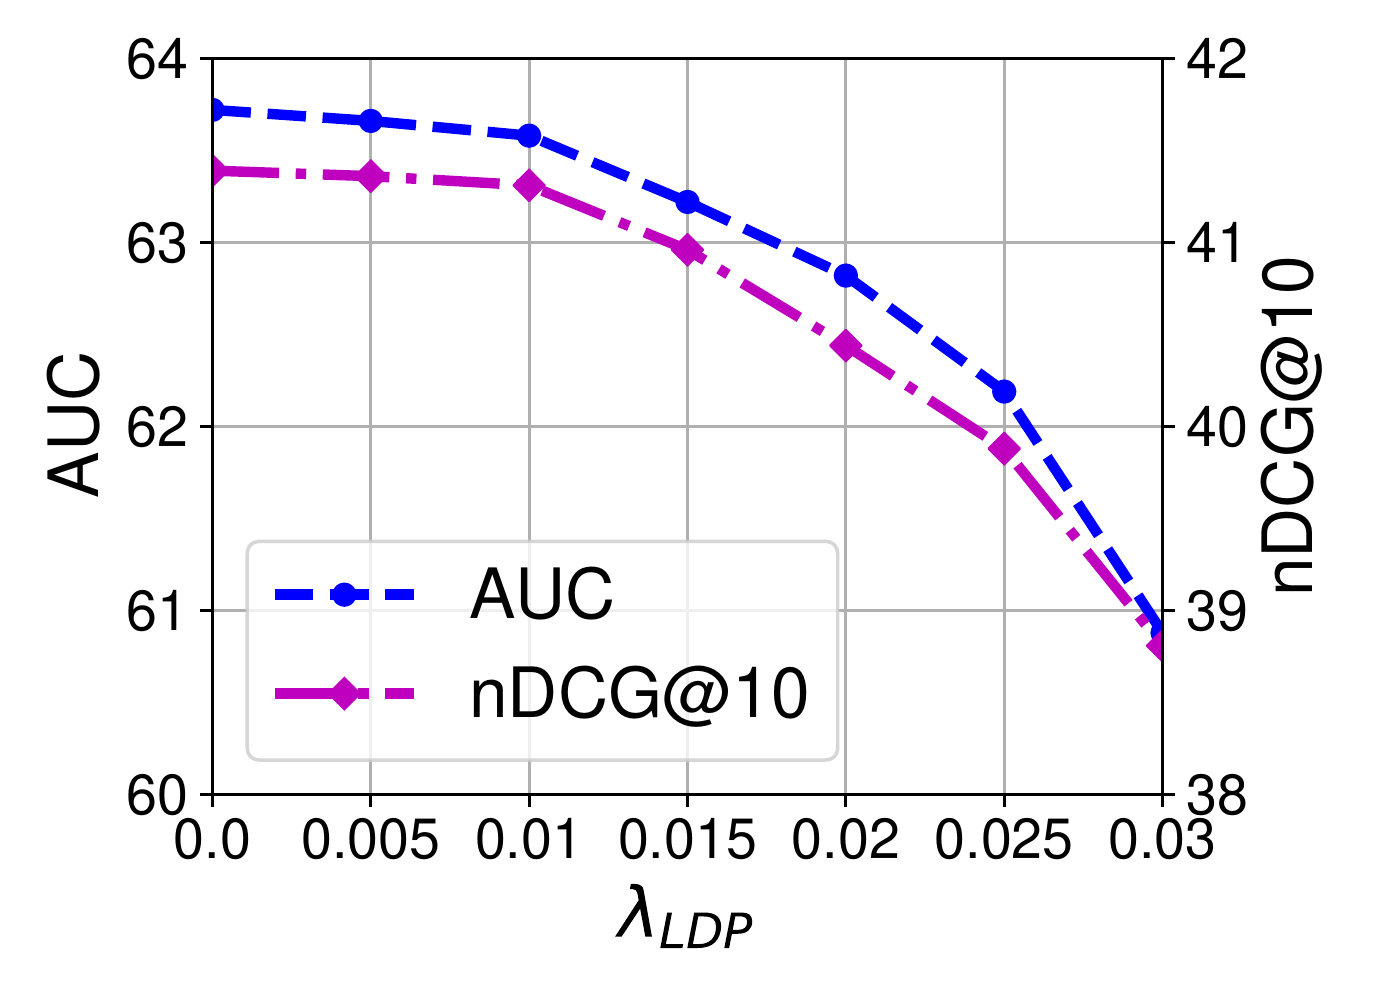}  
    }
    \subfigure[$\lambda_{DP}$.]{
  \includegraphics[width=0.21\textwidth]{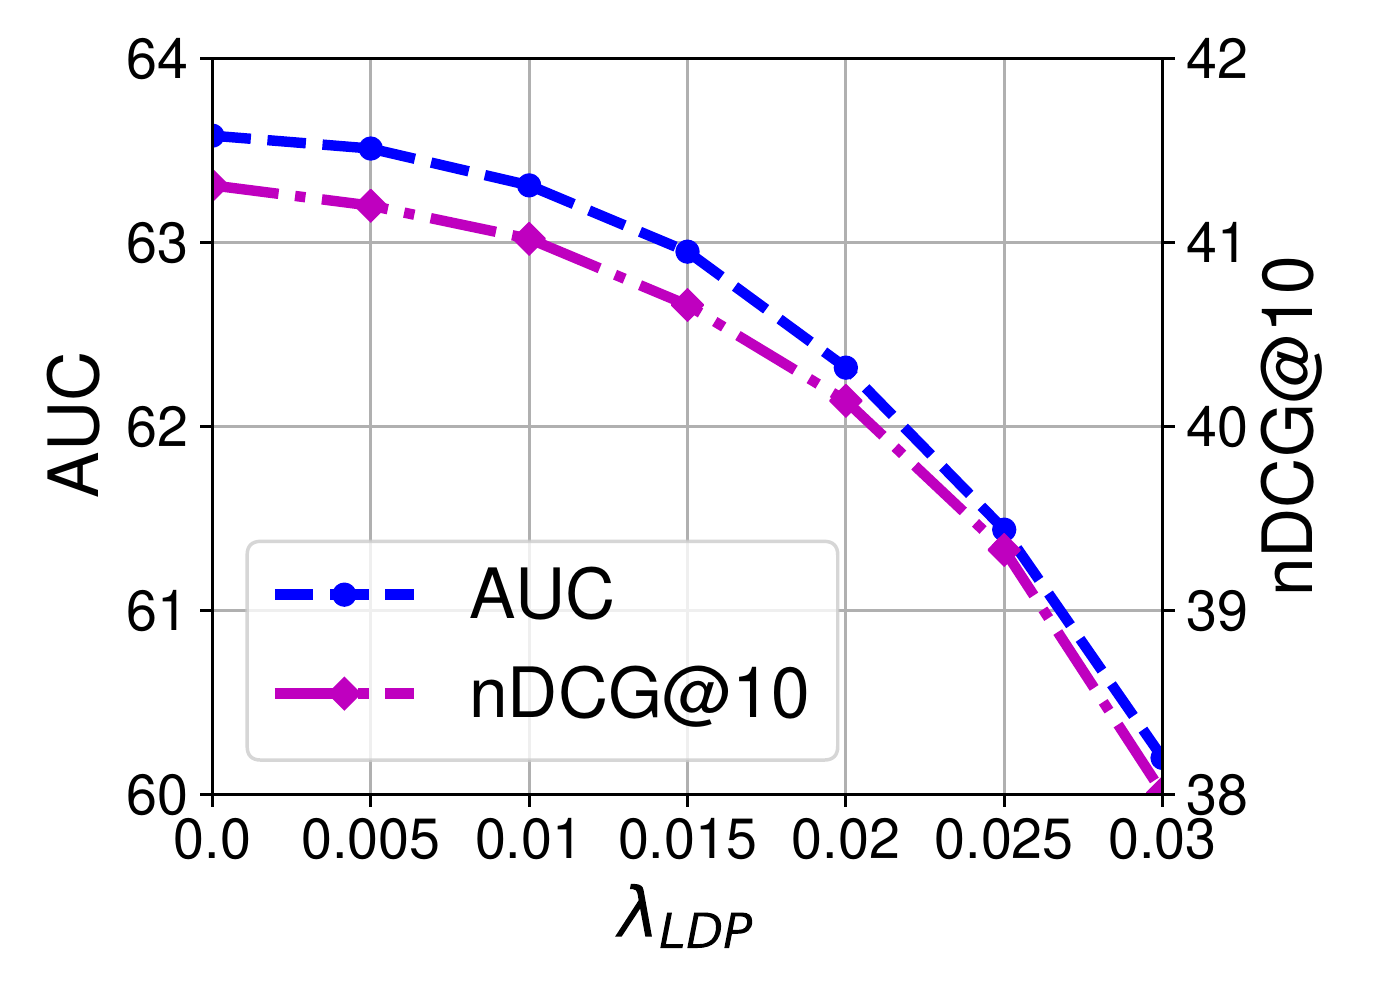}  
    }
 
  \caption{Influence of \small{$\lambda_{LDP}$} and $\lambda_{DP}$ on CTR prediction.} \label{fig.auc3}
 
\end{figure}

We report the results of several experiments on the \textit{News} dataset, which are respectively shown in Figures~\ref{fig.behavior2}, \ref{fig.attack3} and \ref{fig.auc3}.
